# Supplementary material for: The Dispersion Bias
Source: arXiv:1711.05360 source file (2018-02-15)
Supplement: Supplementary file 1 [file lemma.tex]

% -*- root: ../minvar.tex -*-

Throughout this section we will assume a homogeneous risk model $\delta^2 \mat{I}$ 
such that
$$
  \bsig = \sigma_{\nv}^2 \beta \beta^T + \delta^2 \mat{I}.
$$
Also all estimated quantities, $\hat\sigma_{\nv}^2$, $\hat\beta$, $\hat\delta^2$
are general and not necessarily the PCA estimates.

As in \ci{clarke2011}, define the minimum variance long-short threshold as
\begin{align*}\label{eq:mvls}
  \beta_\mvls
     = \frac{ \vf + \delta^2 }{ \sqrt{\nv}\gamma_{\beta, z} \vf},
\end{align*}
where an analogous term $\wh{\beta}_\mvls$ is defined using estimated
quantities.  Further, as in \ci{clarke2011}, let $w$ and 
$\bar{w}$ stand for the
normalized and unnormalized weights of the minimum variance portfolio given by,
\begin{gather}
  w = \frac{\beta_{\mvls} - \beta}{\nv\beta_{\mvls} - \sqrt{\nv}\gamma_{\beta, z}}
    = \frac{
      \frac{\sigma^2 + \delta^2}{\sqrt{\nv}\gamma_{\beta, z}\sigma^2} - \beta
    }{
      {\sqrt{\nv}}
      \left( 
        \frac{\sigma^2 + \delta^2}
          {\gamma_{\beta, z}\sigma^2} - \gamma_{\beta, z} 
      \right)
    },\\
  \bar{w} = {\beta_{\mvls} - \beta} 
    = \frac{\sigma^2 + \delta^2}{\sqrt{\nv}\gamma_{\beta, z} \sigma^2} - \beta
\end{gather}
As before, analogous quantities $\wh{w}$ and $\wh{\bar{w}}$ are defined using
estimated quantities.

The following lemmas establish fundamental building blocks for analyzing
tracking error and forecast variance ratio.  As  above, a formula in terms of true quantities has an analog
in terms of estimated quantities.
%wherever we provide a formula in terms of quantities that do not contain
%estimated quantities, an analogous formula exists using estimated quantities
Further, our  factor model specification implies
$\sigma_{\nv}^2 = \mathcal{O}(\nv)$.  The lemmas are presented without proofs
since they are straightforward to verify from the formulas given above and the asymptotic nature of
$\sigma_{\nv}^2$.

\begin{lemma} \label{L:1}
  \begin{align*}
    w^T w
       % & = \frac{
       %      \beta_\mvls^2 {\nv} - 2 \beta_\mvls \sqrt{\nv}\gamma_{\beta, z} + 1
       %    }{
       %      \left(\nv\beta_\mvls - \sqrt{\nv}\gamma_{\beta, z}\right)^2
       %    } \\
       & = \frac{
            \left(\frac{\frac{\delta^2}{\sigma_{\nv}^2} + 1}{\gamma_{\beta, z}}\right)^2 
              - 2 \left(\frac{\delta^2}{\sigma_{\nv}^2} + 1\right)
              + 1 
          }{
            {\nv}
            \left( 
              \frac{\frac{\delta^2}{\sigma_{\nv}^2} + 1}{\gamma_{\beta, z}}
                 - \gamma_{\beta, z} 
            \right)^2
          }, \\
       & \sim \frac{ 1 }{ 1 - \gamma_{\beta, z}^2 }, 
            \quad \nv \rightarrow \infty \\
    \bar{w}^T \bar{w}
       % & = \beta_\mvls^2 {\nv} 
       %  - 2 \beta_\mvls \sqrt{\nv}\gamma_{\beta, z} + 1 \\
       & = \left(\frac{\frac{\delta^2}{\sigma_{\nv}^2} + 1}{\gamma_{\beta, z}}\right)^2 
          - 2 \left(\frac{\delta^2}{\sigma_{\nv}^2} + 1\right)
          + 1 \\
       & \sim \frac{ 1 - \gamma_{\beta, z}^2 }{ \gamma_{\beta, z}^2 }, 
            \quad \nv \rightarrow \infty,\\
    \wh{w}^T w
       & = \frac{
            \frac{1}{\gamma_{\beta, z}\gamma_{\eb, z}}
              \left(\frac{\delta^2}{\sigma_{\nv}^2} + 1\right)
                \left(\frac{\hat\delta^2}{\hat\sigma_{\nv}^2} + 1\right)
          }{
            {\nv}
              \left( 
                \frac{\frac{\delta^2}{\sigma_{\nv}^2} + 1}{\gamma_{\beta, z}}
                   - \gamma_{\beta, z} 
              \right)
              \left( 
                \frac{\frac{\hat\delta^2}{\hat\sigma_{\nv}^2} + 1}{\gamma_{\eb, z}}
                   - \gamma_{\eb, z} 
              \right)
          } \\
       & \quad + \frac{
            \gamma_{\beta, \eb}
            - \frac{\gamma_{\beta, z}}{\gamma_{\eb, z}}
                \left(\frac{\hat\delta^2}{\hat\sigma_{\nv}^2} + 1\right) 
            - \frac{\gamma_{\eb, z}}{\gamma_{\beta, z}}
                \left(\frac{\delta^2}{\sigma_{\nv}^2} + 1\right)
          }{
            {\nv}
              \left( 
                \frac{\frac{\delta^2}{\sigma_{\nv}^2} + 1}{\gamma_{\beta, z}}
                   - \gamma_{\beta, z} 
              \right)
              \left( 
                \frac{\frac{\hat\delta^2}{\hat\sigma_{\nv}^2} + 1}{\gamma_{\eb, z}}
                   - \gamma_{\eb, z} 
              \right)
          }\\
       & \sim \frac{
            1 - \gamma_{\eb, z}^2 - \gamma_{\beta, z}^2
              + \gamma_{\beta, z}\gamma_{\eb, z}\gamma_{\beta, \eb}
          }{
            \nv
            (1 - \gamma_{\eb, z}^2)
            (1 - \gamma_{\beta, z}^2)
          }
  \end{align*}

\end{lemma}

\begin{lemma} \label{L:2}

  \begin{align*}
    {w}^T \beta 
       & = \frac{
              {\delta^2} / {\sigma_{\nv}^2}
            }{
              \sqrt{\nv}
              \left( 
                \frac{\frac{\delta^2}{\sigma_{\nv}^2} + 1}{\gamma_{\beta, z}} 
                   - \gamma_{\beta, z} 
              \right)
            } \\
       & \sim \frac{\delta^2}{\sqrt{\nv}\sigma_{\nv}^2}
              \frac{\gamma_{\beta, z}}{1 - \gamma_{\beta, z}},
                \quad \nv \rightarrow \infty \\
    \bar{w}^T \beta & = \frac{\delta^2}{\sigma_{\nv}^2}
  \end{align*}

\end{lemma}

\begin{lemma} \label{L:3}
  \begin{align*}
    \wh{w}^T \beta 
       & = \frac{
              \frac{\hat\delta^2}{\hat\sigma_{\nv}^2}r_{\hat\beta}
               + ( r_{\hat\beta} - \gamma_{\beta, \eb} )
          }{
            {\sqrt{N}}
            \left( 
              \frac{\frac{\hat\delta^2}{\hat\sigma_{\nv}^2} + 1}
                  {\gamma_{\eb, z}} - \gamma_{\eb, z} 
            \right)
          } \\
       & \sim \frac{1}{\sqrt{N}}
            \frac{ \gamma_{\eb, z} }{ 1 - \gamma_{\eb, z}^2 }
            \left( r_{\hat\beta} - \gamma_{\beta, \eb} \right),
              \quad \nv \rightarrow \infty \\
    \wh{\bar{w}}^T \beta
       & = \frac{\hat\delta^2}{\hat\sigma_{\nv}^2}r_{\eb}
           + (r_{\hat\beta} - \gamma_{\beta, \eb}) \\
       & \sim r_{\hat\beta} - \gamma_{\beta, \eb}, 
            \quad \nv \rightarrow \infty
  \end{align*}

\end{lemma}

\begin{lemma}[In-Sample Factor Risk] \label{L:is_factor_risk}

  \begin{align*}
    \hat\sigma_{\nv}^2 \wh{w}^T \eb\eb^T \wh{w} 
      & = \frac{ \frac{ \hat\delta^4 }{ \hat\sigma_{\nv}^2 } }{
            {\nv}
            \left( 
              \frac{
                \frac{ \hat\delta^2 }{ \hat\sigma_{\nv}^2 } + 1
              }{
                \gamma_{\beta, z}
              } - \gamma_{\beta, z}
            \right)^2
          } \\
      & \sim \frac{ \hat\delta^4 }{ \nv\hat\sigma_{\nv}^2 } 
          \frac{ \gamma_{\beta, z}^2 }{ (1 - \gamma_{\beta, z}^2)^2 },
          \quad \nv \rightarrow \infty \\
    \hat\sigma_{\nv}^2 \wh{\bar{w}}^T \eb\eb^T \wh{\bar{w}}
      & = \frac{ \hat\delta^4 }{ \hat\sigma_{\nv}^2 } \\
  \end{align*}

\end{lemma}

\begin{lemma}[Out-of-Sample Factor Risk] \label{L:oos_factor_risk}

  \begin{align*}
    \sigma_{\nv}^2 \wh{w}^T \beta\beta^T \wh{w} 
      & = {\sigma_{\nv}^2} 
          \left(
            \frac{
              \frac{\hat\delta^2}{\hat\sigma_{\nv}^2}r_{\hat\beta}
               + (r_{\eb} - \gamma_{\beta, \eb})
            }{
              {\sqrt{N}}
              \left( 
                \frac{\frac{\hat\delta^2}{\hat\sigma_{\nv}^2} + 1}
                    {\gamma_{\eb, z}} - \gamma_{\eb, z} 
              \right)
            }
          \right)^2 \\
      & \sim \frac{\sigma_{\nv}^2}{N}
          \frac{ \gamma_{\eb, z}^2 }{ (1 - \gamma_{\eb, z}^2)^2 }
          \left( r_{\eb} - \gamma_{\beta, \eb} \right)^2,
          \quad \nv \rightarrow \infty \\
    \sigma_{\nv}^2 \wh{\bar{w}}^T \beta\beta^T \wh{\bar{w}} 
      & = {\sigma_{\nv}^2}\left(
        \frac{\hat\delta^2}{\hat\sigma_{\nv}^2}r_{\eb}
         + (r_{\eb} - \gamma_{\beta, \eb})
          \right)^2 \\
      & \sim {\sigma_{\nv}^2}\left(r_{\eb} - \gamma_{\beta, \eb}\right)^2,
          \quad \nv \rightarrow \infty
  \end{align*}

\end{lemma}

\begin{corollary}[Out-of-Sample Factor Risk] \label{Cor:oos_factor_risk}
  Let $\eb \in \mathcal{S}_\beta$.
  \begin{align*}
    \sigma_{\nv}^2 \wh{w}^T \beta\beta^T \wh{w} 
      & = {\sigma_{\nv}^2} 
          \left(
            \frac{
              \frac{\hat\delta^2}{\hat\sigma_{\nv}^2}r_{\hat\beta}
            }{
              {\sqrt{N}}
              \left( 
                \frac{\frac{\hat\delta^2}{\hat\sigma_{\nv}^2} + 1}
                    {\gamma_{\eb, z}} - \gamma_{\eb, z} 
              \right)
            }
          \right)^2 \\
      & \sim \frac{\sigma_{\nv}^2}{N}
          \frac{ \gamma_{\eb, z}^2 }{ (1 - \gamma_{\eb, z}^2)^2 }
          \frac{\hat\delta^4}{\hat\sigma_{\nv}^4}r_{\hat\beta}^2,
          \quad \nv \rightarrow \infty \\
    \sigma_{\nv}^2 \wh{\bar{w}}^T \beta\beta^T \wh{\bar{w}} 
      & = {\sigma_{\nv}^2}\left(
        \frac{\hat\delta^2}{\hat\sigma_{\nv}^2}r_{\eb}
          \right)^2 \\
      & \sim \frac{\hat\delta^4}{\hat\sigma_{\nv}^2}r_{\eb}^2,
          \quad \nv \rightarrow \infty
  \end{align*}

\end{corollary}

\begin{lemma}[In-Sample Specific Risk] \label{L:is_specific_risk}

  \begin{align*}
    \wh{w}^T \wh{\bdel} \wh{w}
       & = \hat\delta^2\frac{
            \left(\frac{\frac{\delta^2}{\sigma_{\nv}^2} + 1}{\gamma_{\beta, z}}\right)^2 
              - 2 \left(\frac{\delta^2}{\sigma_{\nv}^2} + 1\right)
              + 1 
          }{
            {\nv}
            \left( 
              \frac{\frac{\delta^2}{\sigma_{\nv}^2} + 1}{\gamma_{\beta, z}}
                 - \gamma_{\beta, z} 
            \right)^2
          }, \\
       & \sim \frac{ \hat\delta^2 }{ 1 - \gamma_{\beta, z}^2 }, 
            \quad \nv \rightarrow \infty \\
    \wh{\bar{w}}^T \wh{\bdel} \wh{\bar{w}}
       & = \hat\delta^2 \left(
            \left(\frac{\frac{\delta^2}{\sigma_{\nv}^2} + 1}{\gamma_{\beta, z}}\right)^2 
              - 2 \left(\frac{\delta^2}{\sigma_{\nv}^2} + 1\right)
              + 1 
          \right) \\
       & \sim \hat\delta^2
            \frac{ 1 - \gamma_{\beta, z}^2 }{ \gamma_{\beta, z}^2 }, 
            \quad \nv \rightarrow \infty
  \end{align*}

\end{lemma}

\begin{lemma}[Out-of-Sample Specific Risk] \label{L:oos_specific_risk}

  \begin{align*}
    \wh{w}^T {\bdel} \wh{w}
       & = \delta^2\frac{
            \left(\frac{\frac{\delta^2}{\sigma_{\nv}^2} + 1}{\gamma_{\beta, z}}\right)^2 
              - 2 \left(\frac{\delta^2}{\sigma_{\nv}^2} + 1\right)
              + 1 
          }{
            {\nv}
            \left( 
              \frac{\frac{\delta^2}{\sigma_{\nv}^2} + 1}{\gamma_{\beta, z}}
                 - \gamma_{\beta, z} 
            \right)^2
          }, \\
       & \sim \frac{ \delta^2 }{ 1 - \gamma_{\beta, z}^2 }, 
            \quad \nv \rightarrow \infty \\
    \wh{\bar{w}}^T {\bdel} \wh{\bar{w}}
       & = \delta^2 \left(
            \left(\frac{\frac{\delta^2}{\sigma_{\nv}^2} + 1}{\gamma_{\beta, z}}\right)^2 
              - 2 \left(\frac{\delta^2}{\sigma_{\nv}^2} + 1\right)
              + 1 
          \right) \\
       & \sim \delta^2
            \frac{ 1 - \gamma_{\beta, z}^2 }{ \gamma_{\beta, z}^2 }, 
            \quad \nv \rightarrow \infty
  \end{align*}

\end{lemma}

\begin{lemma}[Squared Tracking Error] \label{L:te}

  \begin{align*}
    \te_{\wh{w}}^2 
      & = (\wh{w} - w)^T \bsig (\wh{w} - w) \\
      % & = \wh{w}^T \bsig \wh{w} + w^T \bsig w - 2 \wh{w}^T \bsig w \\
      % & = \sigma^2 \wh{w}^T \beta\beta^T \wh{w} + \wh{w}^T \bdel \wh{w} 
      %     + \sigma^2 {w}^T \beta\beta^T {w} 
      %     + {w}^T \bdel {w} \\
      % & \quad - 2 \sigma^2 \wh{w}^T \beta\beta^T {w} 
      %    - 2 \wh{w}^T \bdel {w} \\
      & \sim \frac{\sigma^2}{\nv}\frac{\gamma_{\hat\beta}^2}{(1 - \gamma_{\hat\beta}^2)^2}
          \left( \frac{\gamma_\beta}{\gamma_{\hat\beta}} - \gamma_{\beta, \eb} \right)^2 
           + {\delta^2} \frac{1}{\nv(1 - \gamma_{\hat\beta}^2)} \\
      & \quad + \frac{\delta^4}{{\nv}\sigma^2}
        \frac{\gamma_\beta^2}{(1 - \gamma_\beta^2)^2} 
           + {\delta^2} \frac{1}{\nv(1 - \gamma_{\beta}^2)} \\
      & \quad - 2 \frac{\sigma^2}{\nv} \left(
          \frac{\gamma_{\hat\beta}}{1 - \gamma_{\hat\beta}^2}
            \left( \frac{\gamma_\beta}{\gamma_{\hat\beta}} - \gamma_{\beta, \eb} \right)
        \right) \left(
          \frac{\delta^2}{\sigma^2} \frac{\gamma_\beta}{1 - \gamma_\beta^2}
        \right) \\
      & \quad - 2 \delta^2 \frac{
        \left(
          1 - \gamma_{\hat\beta}^2 - \gamma_\beta^2
          + \gamma_\beta\gamma_{\hat\beta}\gamma_{\beta, \eb}
        \right)
      }{
        \nv
        {(1 - \gamma_{\beta}^2)}
        {(1 - \gamma_{\hat\beta}^2)}
      } \\
      & \sim 
        \frac{\sigma^2}{\nv}\frac{\gamma_{\hat\beta}^2}{(1 - \gamma_{\hat\beta}^2)^2}
          \left( \frac{\gamma_\beta}{\gamma_{\hat\beta}} - \gamma_{\beta, \eb} \right)^2
          + \delta^2 
          \frac{ \gamma_{\hat\beta}^2 - \gamma_\beta^2 }
            {\nv {(1 - \gamma_{\beta}^2)} {(1 - \gamma_{\hat\beta}^2)}},
        \quad \nv \rightarrow \infty
  \end{align*}

\end{lemma}

\begin{corollary}[Squared Tracking Error] \label{Cor:te}
  Let $\eb \in \mathcal{S}_\beta$.
  \begin{align*}
    \te_{\wh{w}}^2 
      & \sim \delta^2 
          \frac{ \gamma_{\hat\beta}^2 - \gamma_\beta^2 }
            {\nv {(1 - \gamma_{\beta}^2)} {(1 - \gamma_{\hat\beta}^2)}},
        \quad \nv \rightarrow \infty
  \end{align*}

\end{corollary}

\begin{lemma}[Forecast Variance Ratio] \label{L:var_ratio}

  \begin{align*}
    \scrR_{\wh w}
       & = \frac{
          \hat\sigma_{\nv}^2 \wh{\bar{w}}^T \eb\eb^T \wh{\bar{w}} 
            + \wh{\bar{w}}^T \wh{\bdel} \wh{\bar{w}}
        }{
          \sigma_{\nv}^2 \wh{\bar{w}}^T \beta\beta^T \wh{\bar{w}} 
            + \wh{\bar{w}}^T {\bdel} \wh{\bar{w}}
        } \\
       & = \frac{
          \frac{ \hat\delta^4 }{ \hat\sigma_{\nv}^2 } 
            + \hat\delta^2
              \left(
                \left(
                  \frac{\frac{\delta^2}{\sigma_{\nv}^2} + 1}
                    {\gamma_{\eb, z}}
                \right)^2 
                  - 2 \left(\frac{\delta^2}{\sigma_{\nv}^2} + 1\right)
                  + 1
              \right)
        }{
          {\sigma_{\nv}^2}\left(
            \frac{\hat\delta^2}{\hat\sigma_{\nv}^2}r_{\eb}
             + (r_{\eb} - \gamma_{\beta, \eb})
          \right)^2
           + \delta^2 \left(
              \left(
                \frac{\frac{\delta^2}{\sigma_{\nv}^2} + 1}
                  {\gamma_{\eb, z}}
              \right)^2 
                - 2 \left(\frac{\delta^2}{\sigma_{\nv}^2} + 1\right)
                + 1 
            \right)
        } \\
       & \sim \frac{
            \hat\delta^2
        }{
          {\sigma_{\nv}^2}
          \frac{\gamma_{\eb, z}^2}{ (1 - \gamma_{\eb, z}^2)^2}
          \left( r_{\eb} - \gamma_{\beta, \eb} \right)^2
           + \delta^2
        }, \quad \nv \rightarrow \infty
  \end{align*}

\end{lemma}

\begin{corollary}[Forecast Variance Ratio] \label{Cor:var_ratio}
  Let $\eb \in \mathcal{S}_\beta$.
  \begin{align*}
    \scrR_{\wh w}
       & = \frac{
          \frac{ \hat\delta^4 }{ \hat\sigma_{\nv}^2 } 
            + \hat\delta^2
              \left(
                \left(
                  \frac{\frac{\delta^2}{\sigma_{\nv}^2} + 1}
                    {\gamma_{\eb, z}}
                \right)^2 
                  - 2 \left(\frac{\delta^2}{\sigma_{\nv}^2} + 1\right)
                  + 1
              \right)
        }{
          {\sigma_{\nv}^2}\left(
            \frac{\hat\delta^2}{\hat\sigma_{\nv}^2}r_{\eb}
          \right)^2
           + \delta^2 \left(
              \left(
                \frac{\frac{\delta^2}{\sigma_{\nv}^2} + 1}
                  {\gamma_{\eb, z}}
              \right)^2 
                - 2 \left(\frac{\delta^2}{\sigma_{\nv}^2} + 1\right)
                + 1 
            \right)
        } \\
       & \sim \frac{\hat\delta^2}{\delta^2}, \quad \nv \rightarrow \infty
  \end{align*}

\end{corollary}

% \begin{lemma}[Factor Forecast Variance Ratio] \label{L:factor_var_ratio}

%   \begin{align*}
%     \scrR_{\wh w}^{\bell} 
%        & = \frac{
%           \hat\sigma_{\nv}^2 \wh{\bar{w}}^T \eb\eb^T \wh{\bar{w}} 
%         }{
%           \sigma_{\nv}^2 \wh{\bar{w}}^T \beta\beta^T \wh{\bar{w}} 
%         } \\
%        & = \frac{
%           \frac{ \hat\delta^4 }{ \hat\sigma_{\nv}^2 }
%         }{
%           {\sigma_{\nv}^2}\left(
%             \frac{\hat\delta^2}{\hat\sigma_{\nv}^2}r_{\eb}
%              + (r_{\eb} - \gamma_{\beta, \eb})
%           \right)^2
%         } \\
%        & \sim \frac{
%           \frac{ \hat\delta^4 }{ \hat\sigma_{\nv}^2 }
%         }{
%           {\sigma_{\nv}^2}
%           \left( r_{\eb} - \gamma_{\beta, \eb} \right)^2
%         }, \quad \nv \rightarrow \infty
%   \end{align*}

% \end{lemma}

% \begin{corollary}[Factor Forecast Variance Ratio] \label{Cor:factor_var_ratio}
%   Let $\eb \in \mathcal{S}_\beta$.
%   \begin{align*}
%     \scrR_{\wh w}^{\bell} 
%        & = \frac{
%           \frac{ \hat\delta^4 }{ \hat\sigma_{\nv}^2 }
%         }{
%           {\sigma_{\nv}^2}\left(
%             \frac{\hat\delta^2}{\hat\sigma_{\nv}^2}r_{\eb}
%           \right)^2
%         } \\
%        & \sim \frac{ \hat\sigma_{\nv}^2 }{ \sigma_{\nv}^2 r_{\eb}^2 }, 
%           \quad \nv \rightarrow \infty
%   \end{align*}

% \end{corollary}
