# Supplementary material for: The Dispersion Bias
Source: arXiv:1711.05360 source file (2018-02-15)
Supplement: Supplementary file 2 [file tables.tex]

% -*- root: ../minvar.tex -*- 

\begin{subtable}[t]{\linewidth}
    \centering
    \begin{tabular}{lrrrrrr}
\toprule
N &  500  &  1000 &  1500 &  2000 &  2500 &  3000 \\
\midrule
PCA         & 1.10\% & 0.80\% & 0.76\% & 0.69\% & 0.74\% & 0.70\% \\
Oracle      & 0.80\% & 0.48\% & 0.37\% & 0.35\% & 0.33\% & 0.28\% \\
Data-Driven & 0.82\% & 0.49\% & 0.37\% & 0.35\% & 0.32\% & 0.28\% \\
\bottomrule
\end{tabular}

    \caption{Annualized Tracking Error: Minimum Variance}
\end{subtable}

\begin{subtable}[t]{\linewidth}
    \centering
    \begin{tabular}{lrrrrrr}
\toprule
N &  500  &  1000 &  1500 &  2000 &  2500 &  3000 \\
\midrule
PCA         & 2.93\% & 1.99\% & 1.68\% & 1.45\% & 1.39\% & 1.27\% \\
Oracle      & 2.83\% & 1.89\% & 1.54\% & 1.32\% & 1.22\% & 1.10\% \\
Data-Driven & 2.83\% & 1.89\% & 1.54\% & 1.32\% & 1.22\% & 1.10\% \\
\bottomrule
\end{tabular}

    \caption{Annualized Volatility: Minimum Variance}
\end{subtable}

\begin{subtable}[t]{\linewidth}
    \centering
    \begin{tabular}{lrrrrrr}
\toprule
N &  500  &  1000 &  1500 &  2000 &  2500 &  3000 \\
\midrule
PCA         & 0.854 & 0.811 & 0.761 & 0.737 & 0.680 & 0.663 \\
Oracle      & 0.995 & 0.979 & 0.974 & 0.981 & 0.962 & 0.965 \\
Data-Driven & 0.991 & 0.974 & 0.970 & 0.969 & 0.960 & 0.960 \\
\bottomrule
\end{tabular}

    \caption{Forecast Ratio: Minimum Variance}
\end{subtable}

\begin{subtable}[t]{\linewidth}
    \centering
    \begin{tabular}{lrrrrrr}
\toprule
N &  500  &  1000 &  1500 &  2000 &  2500 &  3000 \\
\midrule
PCA         & 1.002 & 0.986 & 0.982 & 1.002 & 0.978 & 1.002 \\
Oracle      & 1.002 & 0.986 & 0.982 & 1.002 & 0.978 & 1.002 \\
Data-Driven & 1.002 & 0.986 & 0.982 & 1.002 & 0.978 & 1.002 \\
\bottomrule
\end{tabular}

    \caption{Forecast Ratio: Equal Weighted}
\end{subtable}

\begin{subtable}[t]{\linewidth}
    \centering
    \begin{tabular}{lrrrrrrr}
\toprule
$\gamma_{\beta, z}$ &  0.50 &  0.60 &  0.70 &  0.80 &  0.90 &  0.95 &  1.00 \\
\midrule
PCA         & 0.25\% & 0.35\% & 0.40\% & 0.58\% & 1.10\% & 1.97\% & 9.09\% \\
Oracle      & 0.23\% & 0.31\% & 0.35\% & 0.49\% & 0.80\% & 1.42\% & 0.54\% \\
Data-Driven & 0.24\% & 0.33\% & 0.37\% & 0.50\% & 0.82\% & 1.43\% & 3.10\% \\
\bottomrule
\end{tabular}

    \caption{Annualized Tracking Error: Minimum Variance}
\end{subtable}

\begin{subtable}[t]{\linewidth}
    \centering
    \begin{tabular}{lrrrrrrr}
\toprule
$\gamma_{\beta, z}$ &  0.50 &  0.60 &  0.70 &  0.80 &  0.90 &  0.95 &   1.00 \\
\midrule
PCA         & 1.34\% & 1.53\% & 1.68\% & 1.89\% & 2.93\% & 4.18\% & 20.17\% \\
Oracle      & 1.33\% & 1.52\% & 1.66\% & 1.87\% & 2.83\% & 3.95\% & 18.02\% \\
Data-Driven & 1.33\% & 1.52\% & 1.67\% & 1.87\% & 2.83\% & 3.95\% & 18.27\% \\
\bottomrule
\end{tabular}

    \caption{Annualized Volatility: Minimum Variance}
\end{subtable}

\begin{subtable}[t]{\linewidth}
    \centering
    \begin{tabular}{lrrrrrrr}
\toprule
$\gamma_{\beta, z}$ &  0.50 &  0.60 &  0.70 &  0.80 &  0.90 &  0.95 &  1.00 \\
\midrule
PCA         & 0.985 & 0.959 & 0.952 & 0.898 & 0.854 & 0.725 & 0.255 \\
Oracle      & 1.015 & 0.994 & 0.993 & 0.982 & 0.995 & 0.970 & 1.020 \\
Data-Driven & 1.011 & 0.992 & 0.987 & 0.968 & 0.991 & 0.957 & 0.928 \\
\bottomrule
\end{tabular}

    \caption{Forecast Ratio: Minimum Variance}
\end{subtable}

\begin{subtable}[t]{\linewidth}
    \centering
    \begin{tabular}{lrrrrrrr}
\toprule
$\gamma_{\beta, z}$ &  0.50 &  0.60 &  0.70 &  0.80 &  0.90 &  0.95 &  1.00 \\
\midrule
PCA         & 1.029 & 1.015 & 0.995 & 1.003 & 1.002 & 1.003 & 1.021 \\
Oracle      & 1.029 & 1.015 & 0.995 & 1.003 & 1.002 & 1.003 & 1.021 \\
Data-Driven & 1.030 & 1.015 & 0.995 & 1.003 & 1.002 & 1.003 & 1.021 \\
\bottomrule
\end{tabular}

    \caption{Forecast Ratio: Equal Weighted}
\end{subtable}
